# Supplementary material for: Comparison of polynomial approximations to speed up planewave-based quantum Monte Carlo calculations
Source: arXiv:1309.6250 source file (2014-10-30)
Supplement: Supplementary file 1 [file supplement.pdf]

# Supplementary Information

**Contents**


**I. Al** 3

A. Varying planewave cutoff 3

1. VMC energy 3
2. VMC RMS energy fluctuation 4
3. VMC kinetic energy 5
4. VMC potential energy 6

B. Varying grid spacing 7

1. VMC energy 7
2. VMC RMS energy fluctuation 8

**II. Si** 9

A. Varying planewave cutoff 9

1. MAE over mean of orbitals 9
2. MAE over mean of orbital gradients 10
3. MAE over mean of orbital Laplacians 11
4. VMC energy 12
5. VMC RMS energy fluctuation 13
6. VMC kinetic energy 14
7. VMC potential energy 15

B. Varying grid spacing 16

1. $\Gamma$ point - VMC energy 16
2. $\Gamma$ point - VMC RMS energy fluctuation 17
3. X point - VMC energy 18
4. X point - VMC RMS energy fluctuation 19
5. L point - VMC energy 20
6. L point - VMC RMS energy fluctuation 21

**III. MgO** 22

A. Varying grid spacing 22

1. VMC energy 22
2. VMC RMS energy fluctuation 23

# I. ALUMINUM

## A. Varying planewave cutoff

### 1. *VMC energy*

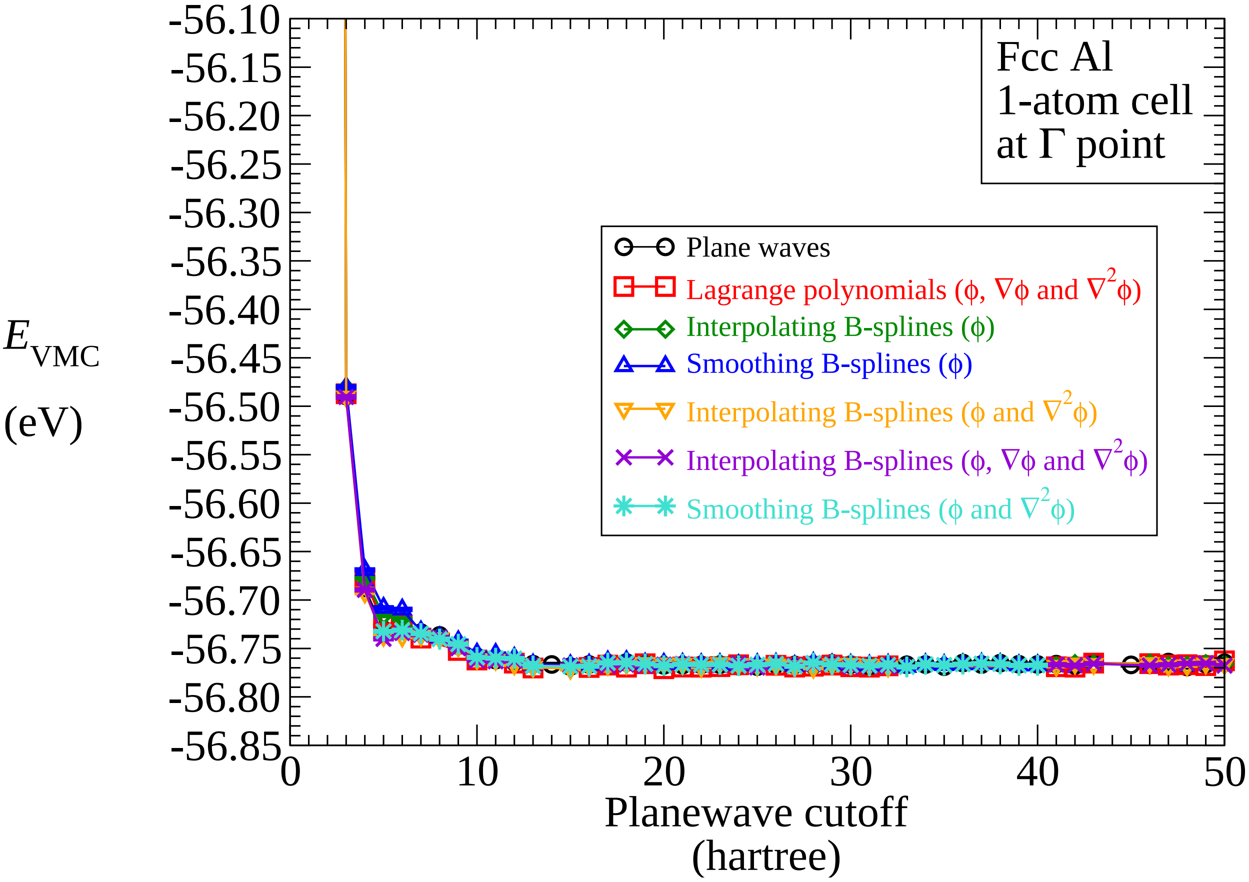


Figure I A 1: Convergence of planewave and approximation-method VMC energies in one-atom fcc Al at the Γ point with planewave basis cutoff energy. 32000 steps on 128 CPUs produced an average uncertainty of 1 meV on the total energy. No method lies outside one standard deviation of the plane wave value at any cutoff depicted.

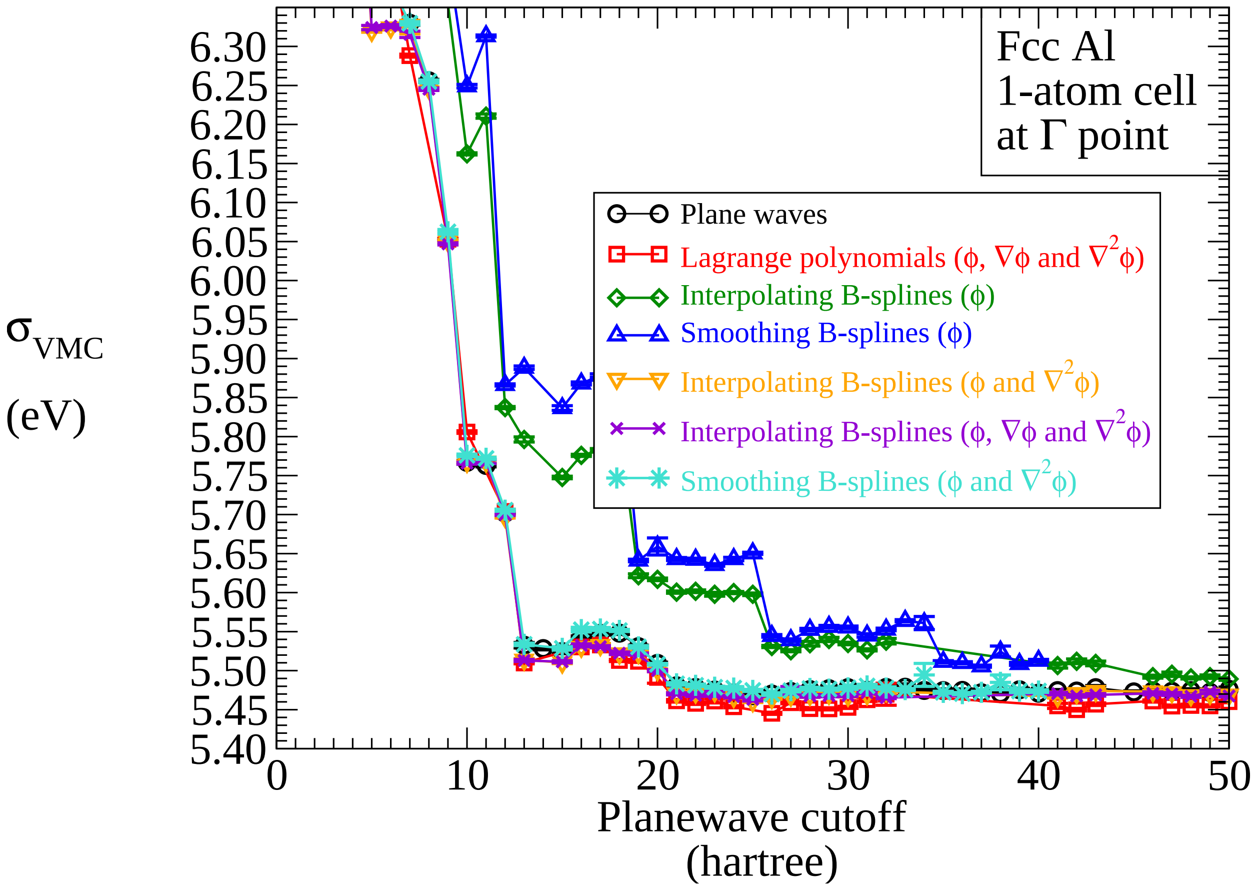


Figure I A 2: Convergence of planewave and approximation-method root-mean-square fluctuations in the VMC energy in one-atom fcc Al at the Γ point with planewave basis cutoff energy. These fluctuation values correspond to the total energies in Figure I A 1. Methods calculating the derivatives of approximations have larger RMS fluctuation than planewaves at small cutoffs. Methods making separate approximation of the planewave Laplacian match the planewave fluctuations in local energy at fixed cutoff.

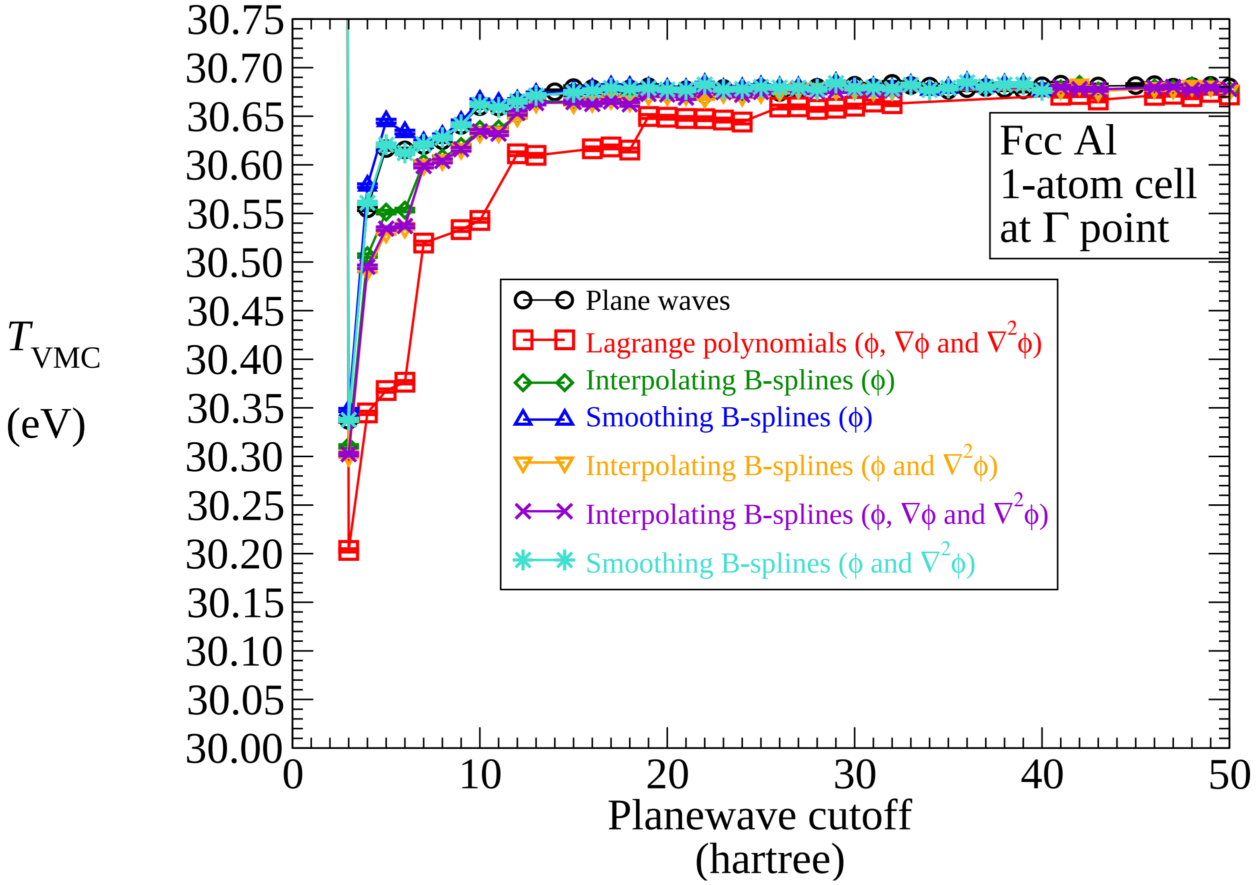


Figure I A 3: Convergence of planewave and approximation-method VMC kinetic energy in one-atom fcc Al at the Γ point with planewave basis cutoff energy. These fluctuation values correspond to the total energies in Figure I A 1. Smoothing B-splines with or without separate approximations for the Laplacian lie closer to the planewave value and reach the converged basis set value at lower cutoff than interpolation methods.

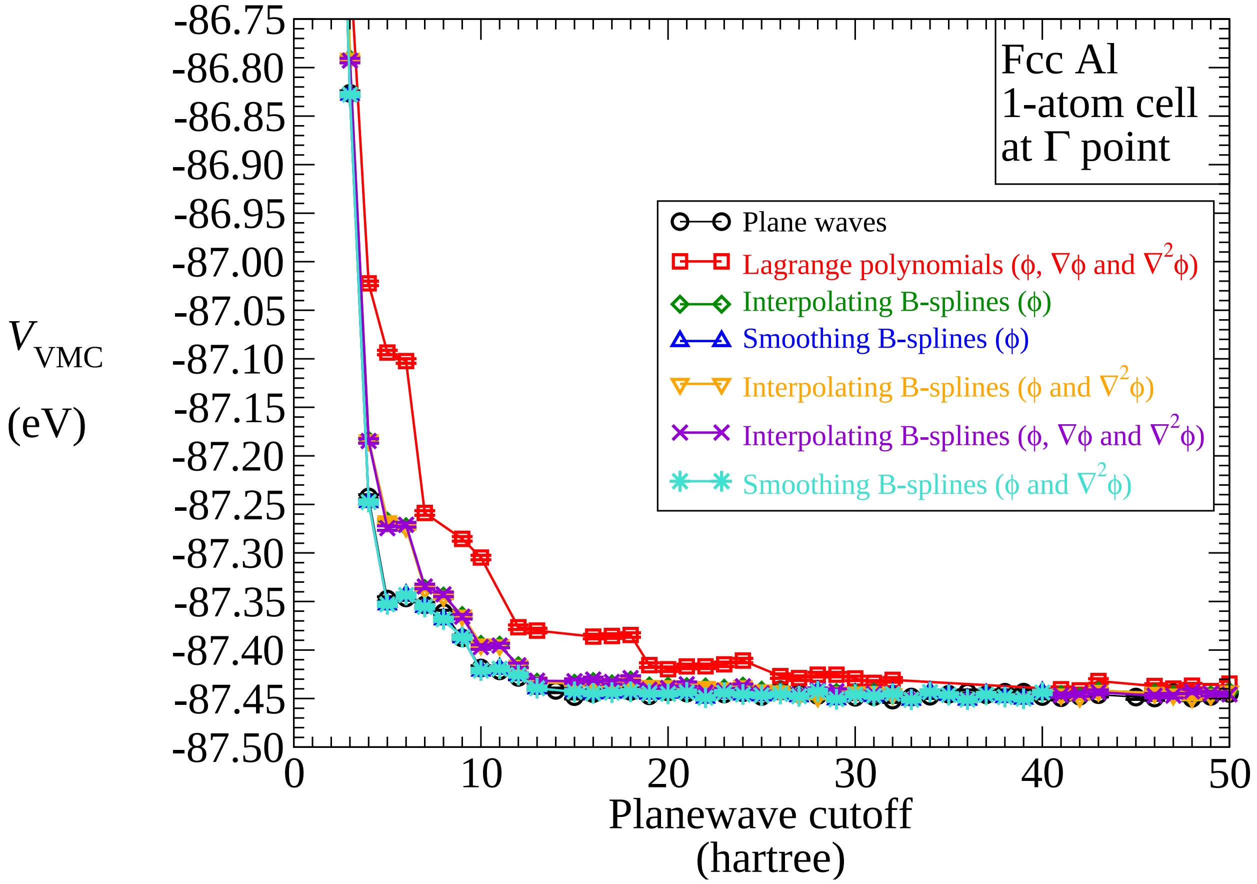


Figure I A 4: Convergence of planewave and approximation-method VMC potential energy in one-atom fcc Al at the Γ point with planewave basis cutoff energy. These fluctuation values correspond to the total energies in Figure I A 1. All B-splines methods lie closer to the planewave value and reach the converged basis set value at lower cutoff than Lagrange polynomials.

## B. Varying grid spacing

### 1. VMC energy

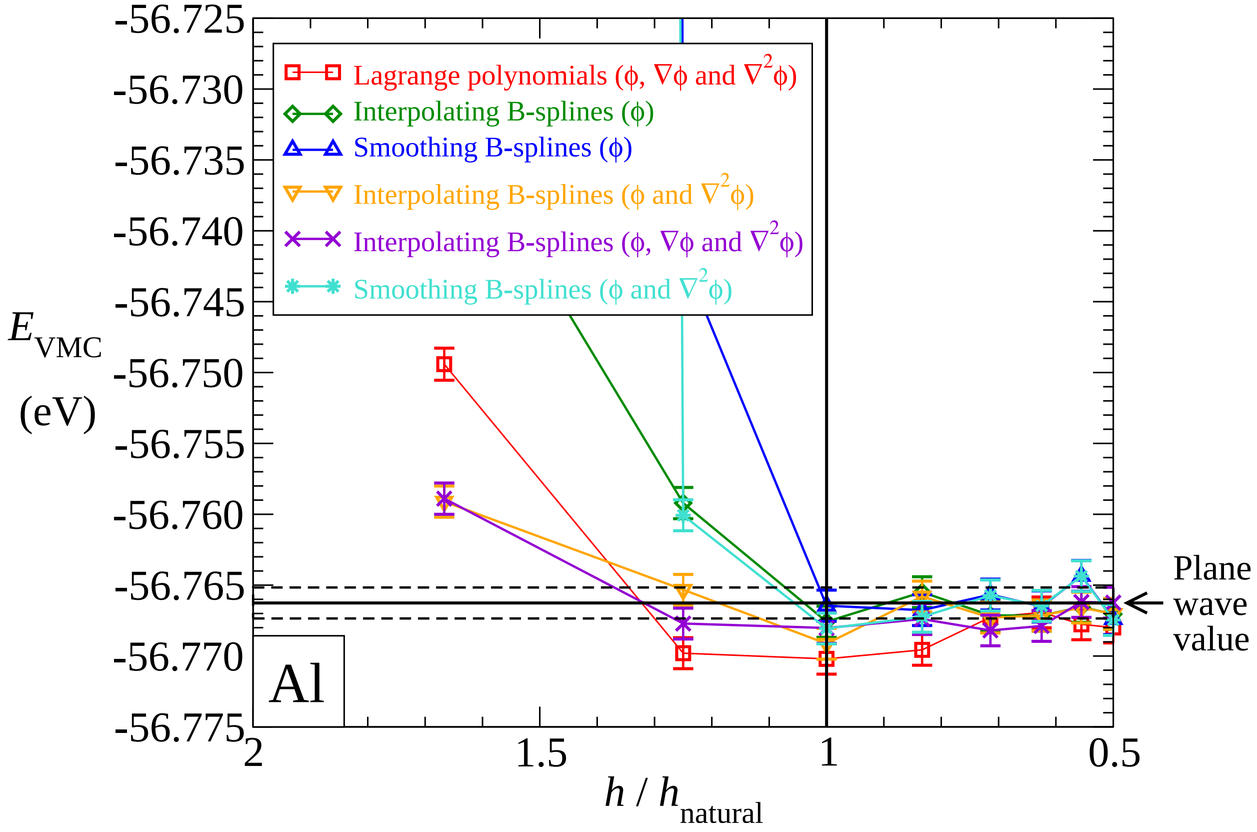


Figure I B 1: Convergence of planewave and approximation-method VMC energies in one-atom fcc Al at the Γ point with grid spacing (given as a ratio to natural grid spacing, defined in Equation 6 of the text). All methods show comparable convergence to the planewave value by natural grid spacing ($h/h_{\mathrm{natural}} = 1$).

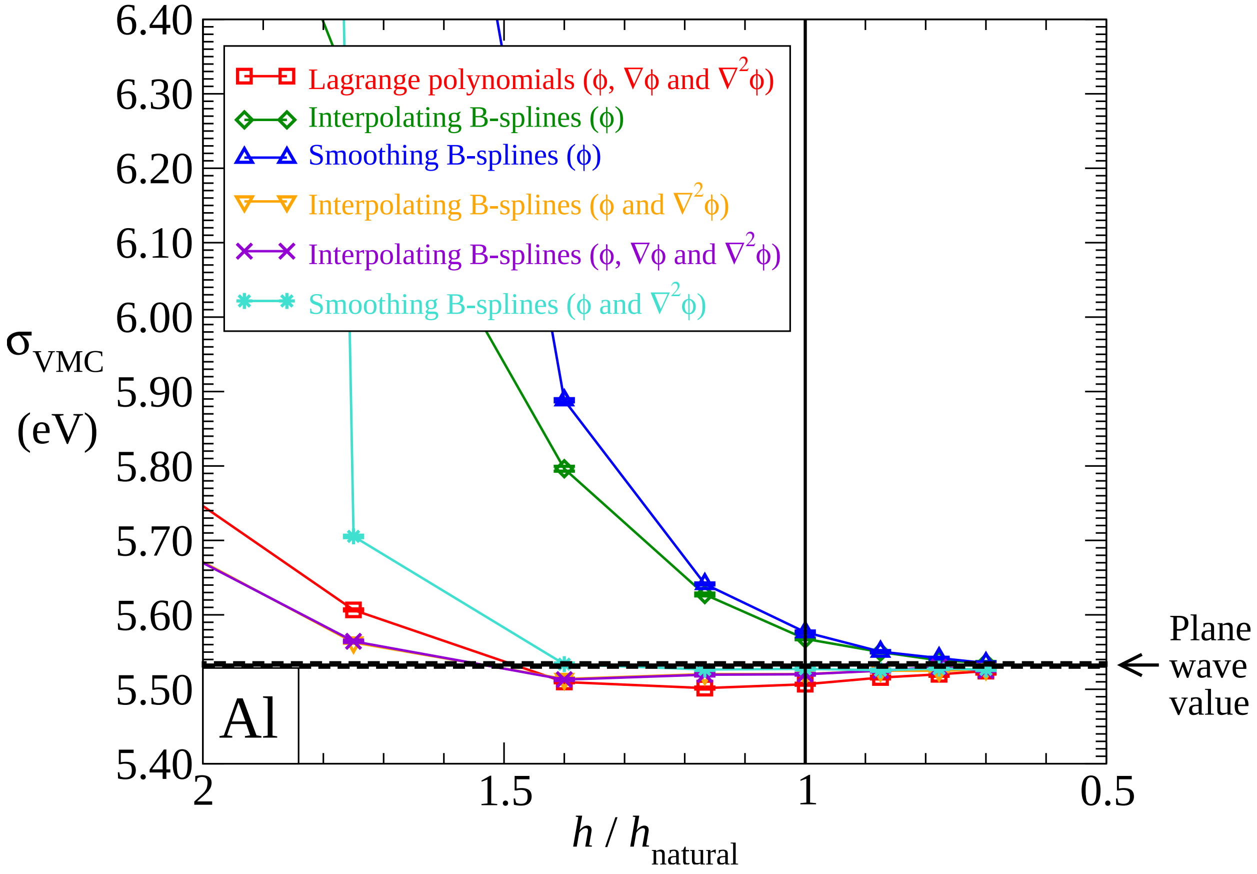


Figure I B 2: Convergence of planewave and approximation-method root-mean-square fluctuation in VMC energy of one-atom fcc Al at the Γ point with grid spacing (given as a ratio to natural grid spacing, defined in Equation 6 of the text). Methods including direct approximation of the orbital Laplacian (those with $\nabla^2\phi$) show convergence to the planewave value at coarser spacings than natural grid spacing. However, methods using derivatives of the approximation to calculate orbital Laplacian (those with $\phi$ alone) converge to the planewave value at finer than natural grid spacing.

## II. SILICON

### A. Varying planewave cutoff

#### 1. *MAE over mean of orbitals*

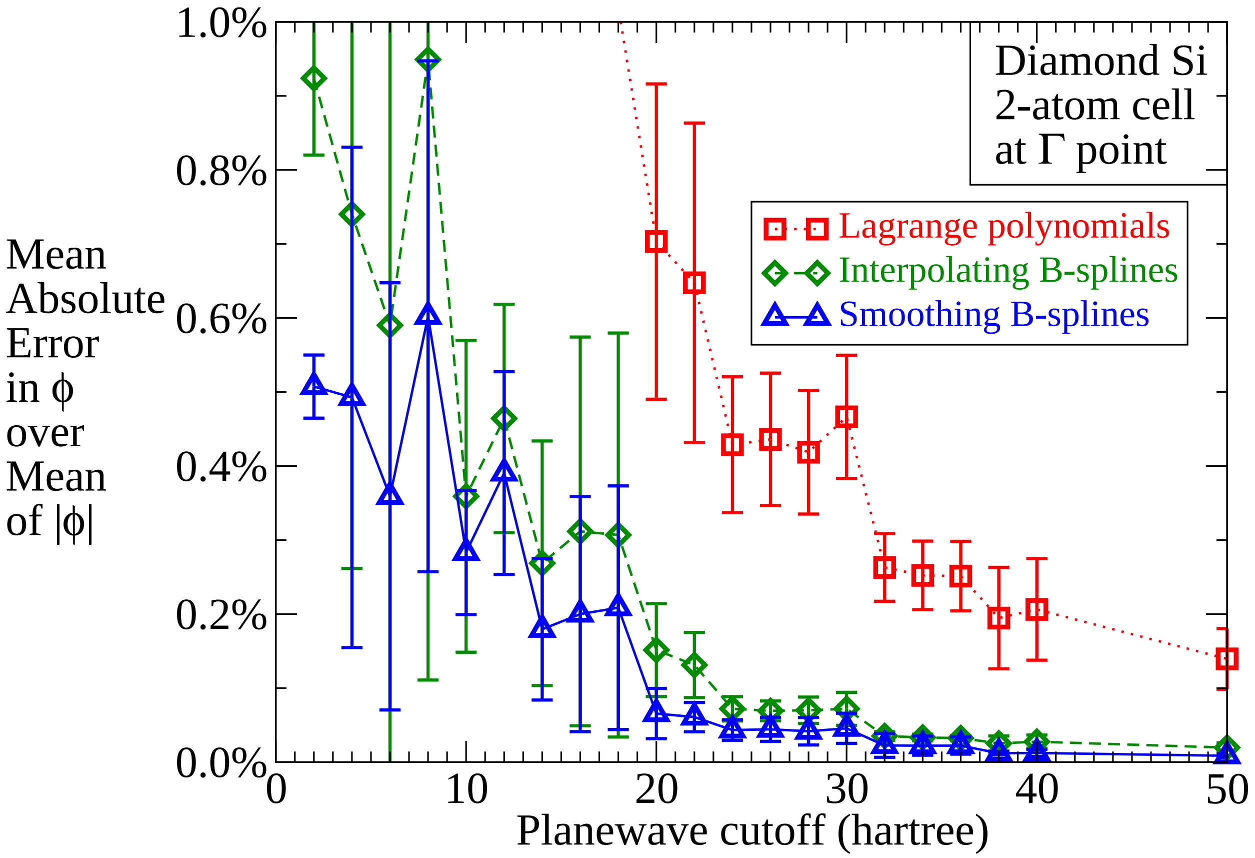


Figure II A 1: Convergence of mean absolute error over mean of approximation methods on the planewave orbitals in two-atom diamond Si at the Γ point with planewave basis cutoff energy. All methods improve with the planewave basis because of the natural grid spacing used. The Lagrange polynomials have a factor of four to six larger error than the two spline methods (interpolating and approximating). The spline methods give comparable results within one standard deviation of their means.

### 2. *MAE over mean of orbital gradients*

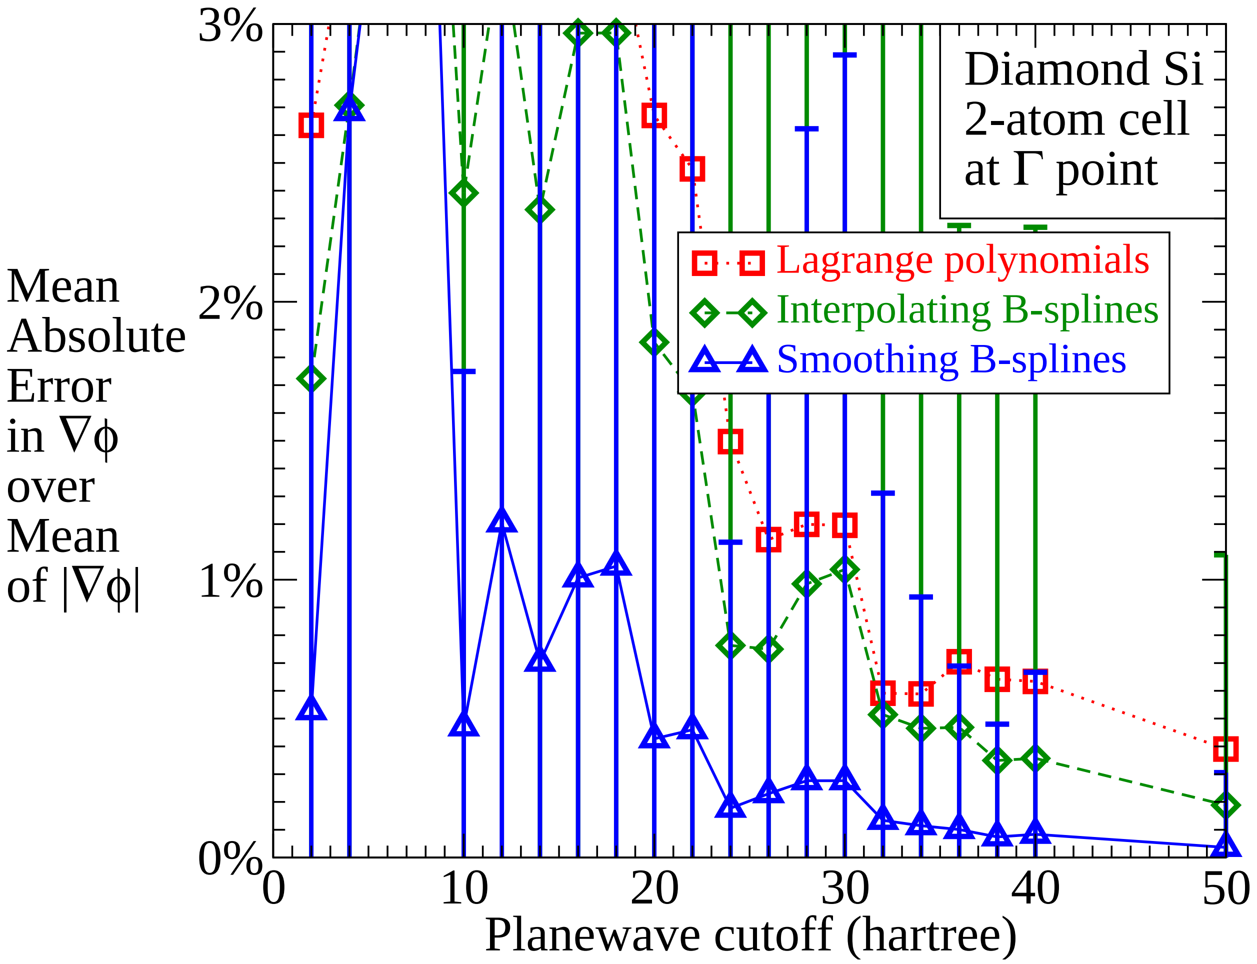


Figure II A 2: Convergence of mean absolute error over mean of approximation methods on the gradient of the planewave orbitals in two-atom diamond Si at the Γ point with planewave basis cutoff energy. All values in this figure use direct approximation of the planewave orbital gradient, not the gradient of the polynomial-approximated orbital. The large standard deviation from averaging the three directions of the gradient obscures the similar trends to the orbital error (depicted in Figure II A 1), even though the absolute percent errors on the gradient are higher than on the orbital itself.

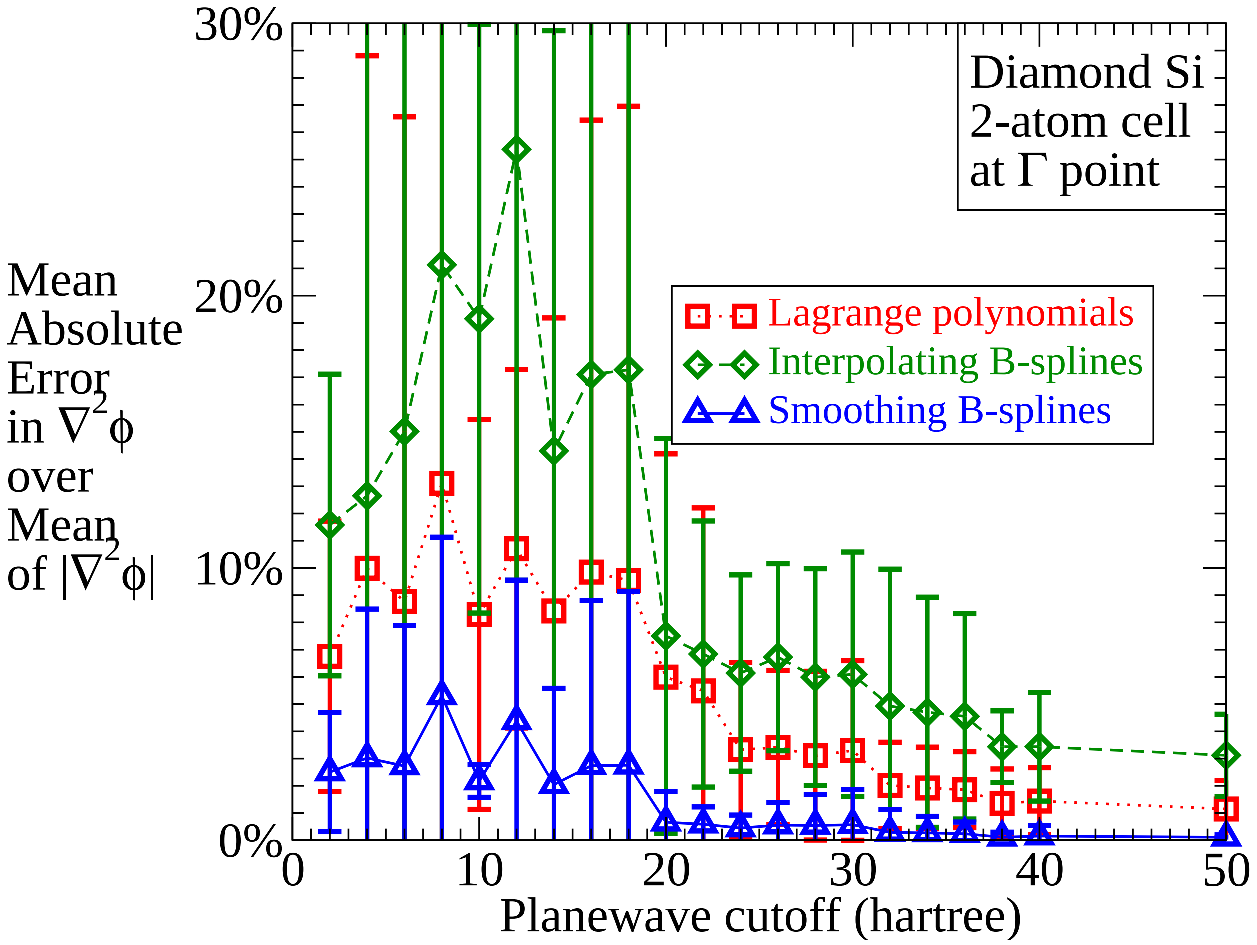


Figure II A 3: Convergence of mean absolute error over mean of approximation methods on the Laplacian of the planewave orbitals in two-atom diamond Si at the Γ point with planewave basis cutoff energy. All values in this figure use direct approximation of the planewave orbital Laplacian, not the Laplacian of the polynomial-approximated orbital. Though the large standard deviation on the values overlaps between each method, the ordering of errors from largest to smallest as Lagrange polynomials, interpolating B-splines, and smoothing B-splines remains for all values of planewave cutoff.

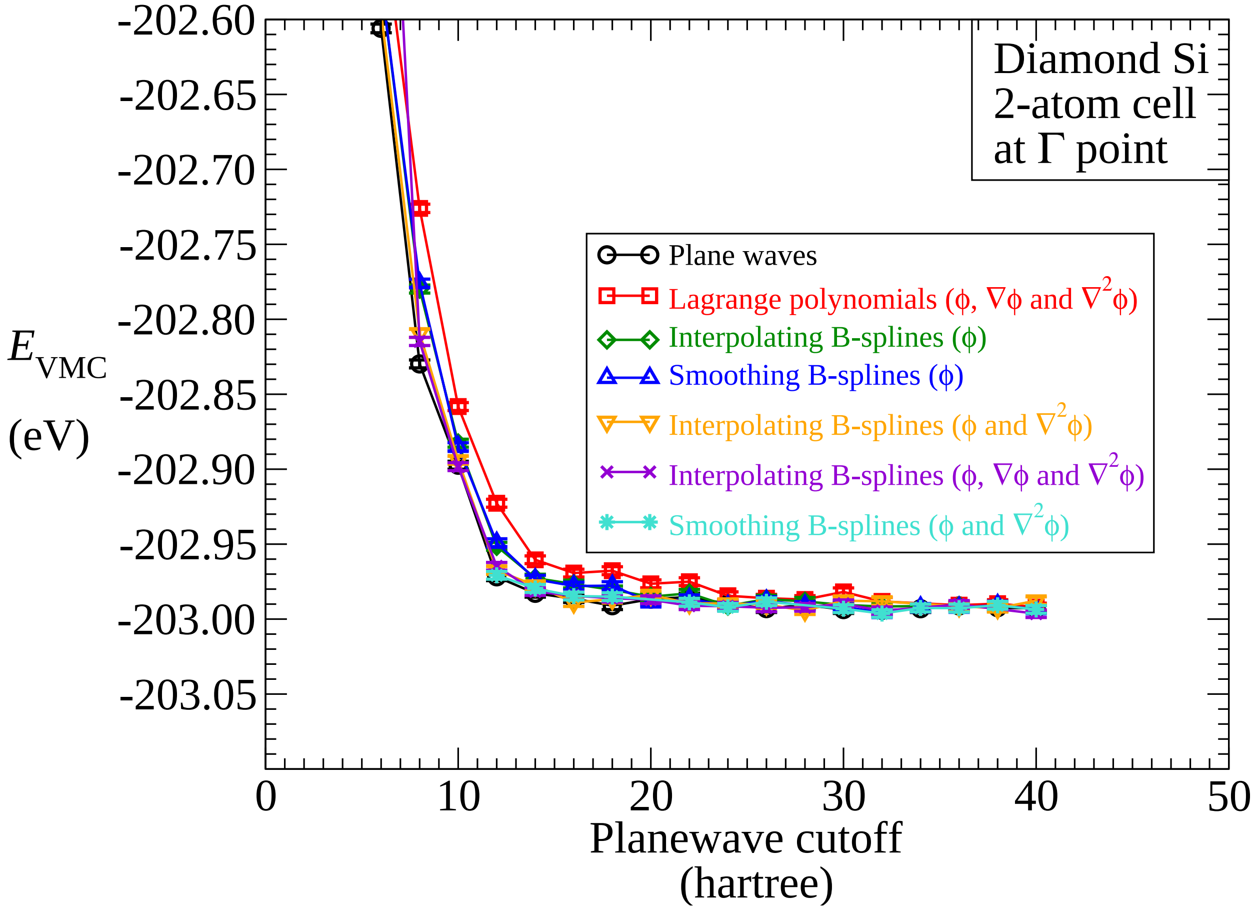


Figure II A 4: Convergence of planewave and approximation-method VMC energies in two-atom diamond Si at the Γ point with planewave basis cutoff energy. 8000 steps on 512 CPUs produced an average uncertainty of 3 meV on the total energy. By the convergence of the VMC energy with planewave cutoff to within its statistical uncertainty near 36 hartree, all methods are within one standard deviation of each other.

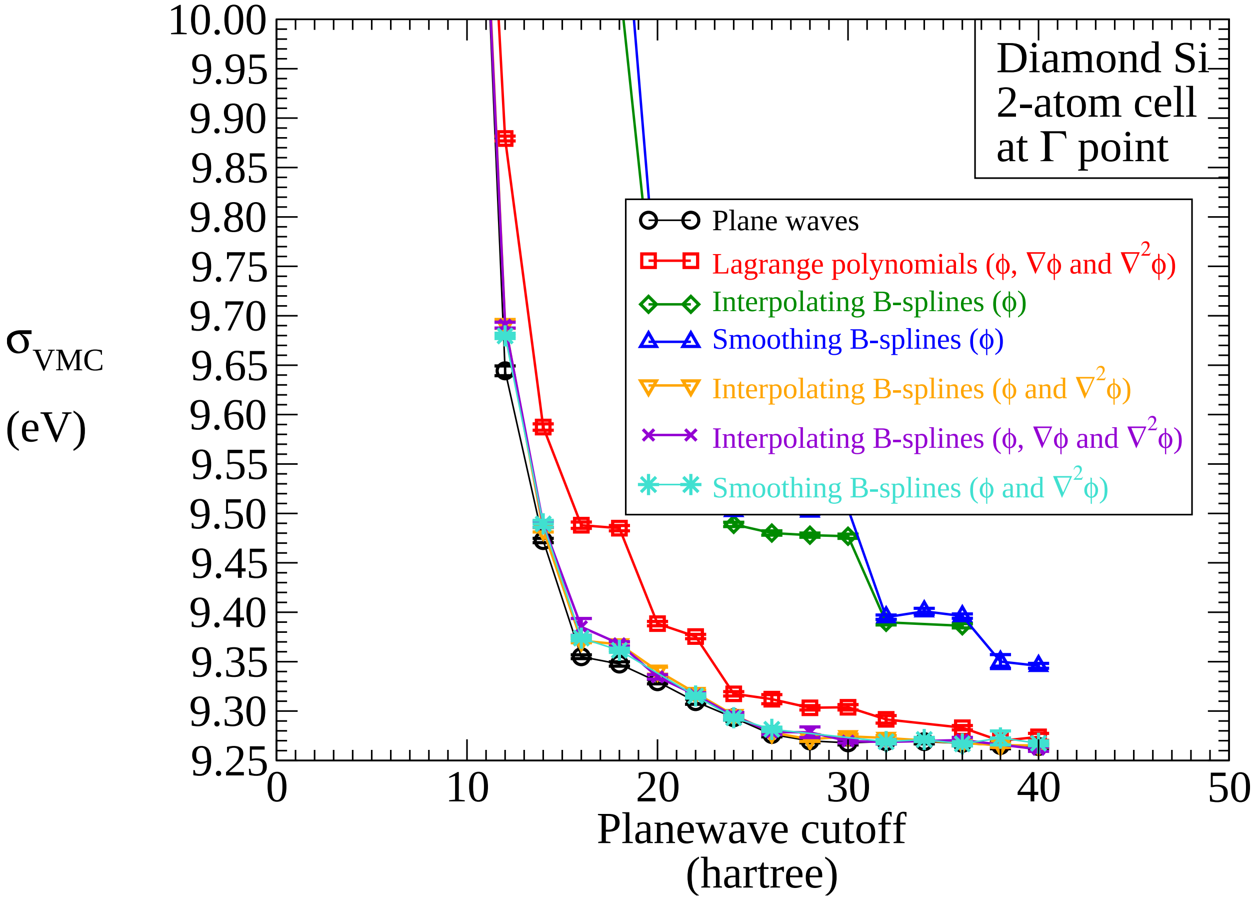


Figure II A 5: Convergence of planewave and approximation-method root-mean-square fluctuations in the VMC energy in two-atom diamond Si at the Γ point with planewave basis cutoff energy. These fluctuation values correspond to the total energies in Figure II A 4. Methods calculating the derivatives of approximations have increased fluctuation compared to planewaves. Lagrange interpolation does not have comparable fluctuation in energy until a cutoff of 38 hartree, 2 hartree above the planewave-converged cutoff. B-splines making separate approximation of the planewave Laplacian (those with $\nabla^2\phi$) match the planewave fluctuations in local energy for fixed cutoff starting at 24 hartree, 12 hartree before the planewave root-mean-square fluctuation has converged.

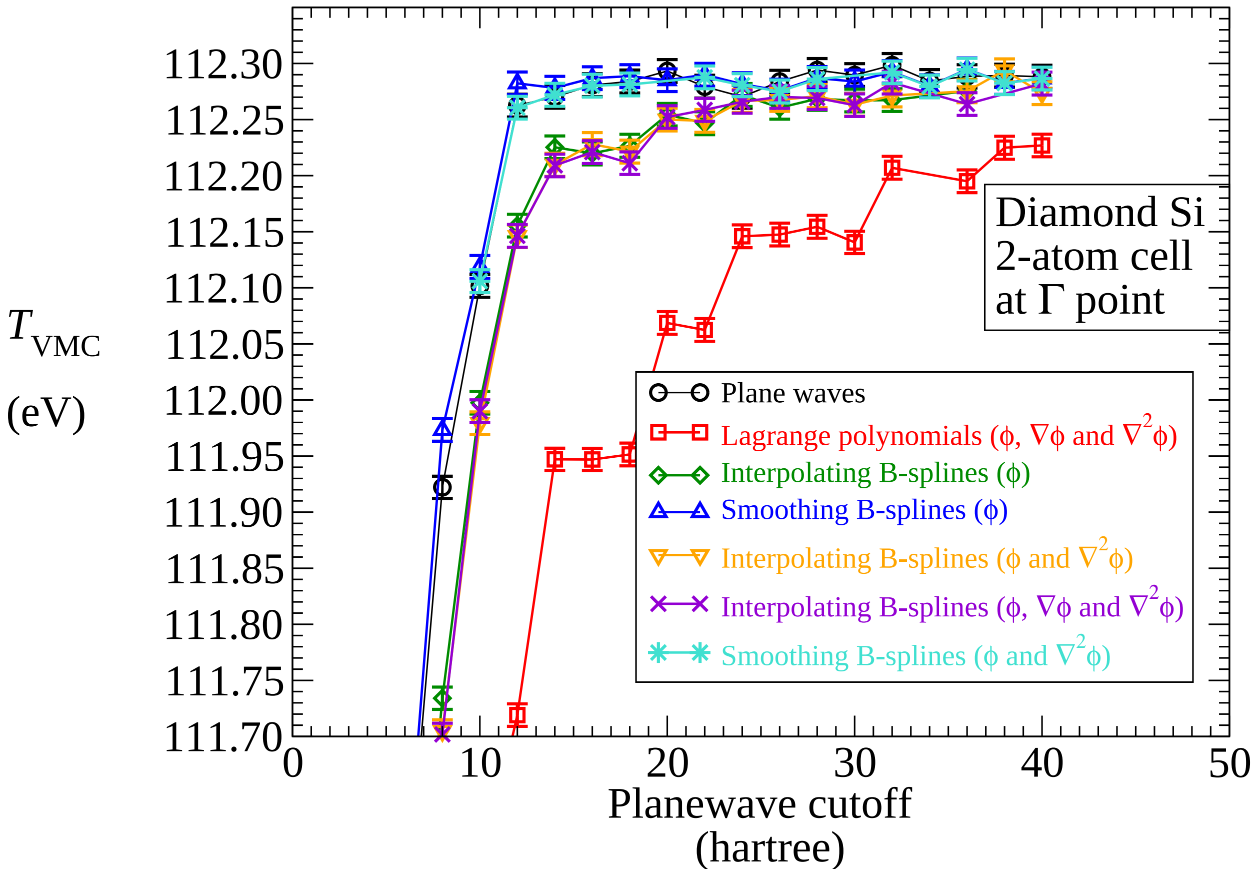


Figure II A 6: Convergence of planewave and approximation-method VMC kinetic energy in two-atom diamond Si at the Γ point with planewave basis cutoff energy. These kinetic energy values correspond to the total energies in Figure II A 4. Smoothing B-splines with or without separate approximation for the Laplacian lie closer to the planewave value and reach the converged basis set value at lower cutoff than interpolation methods.

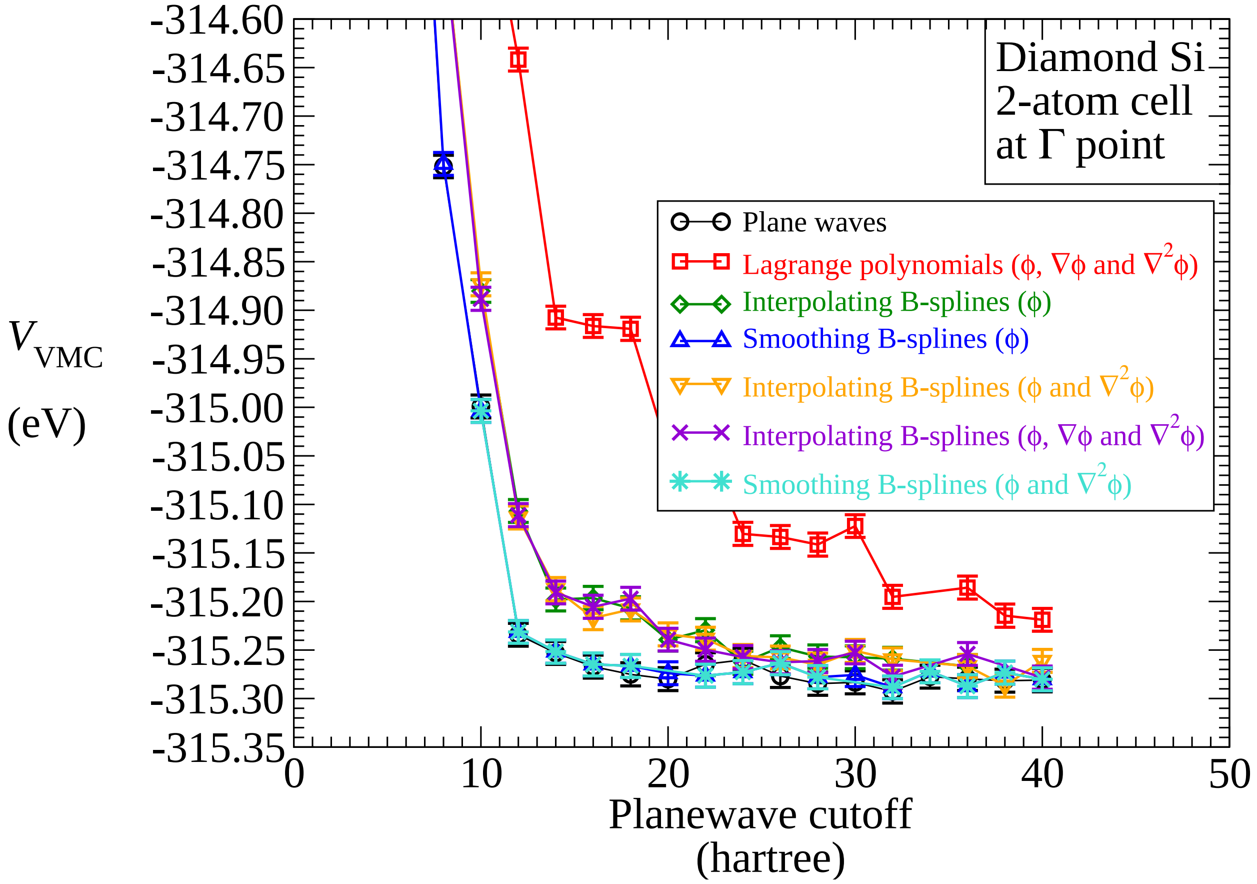


Figure II A 7: Convergence of planewave and approximation-method VMC potential energy in two-atom diamond Si at the Γ point with planewave basis cutoff energy. These potential energy values correspond to the total energies in Figure II A 4. Smoothing B-splines with or without separate approximation for the Laplacian lie closer to the planewave value and reach the converged basis set value at lower cutoff than interpolation methods.

## B. Varying grid spacing

### 1. Γ point - VMC energy

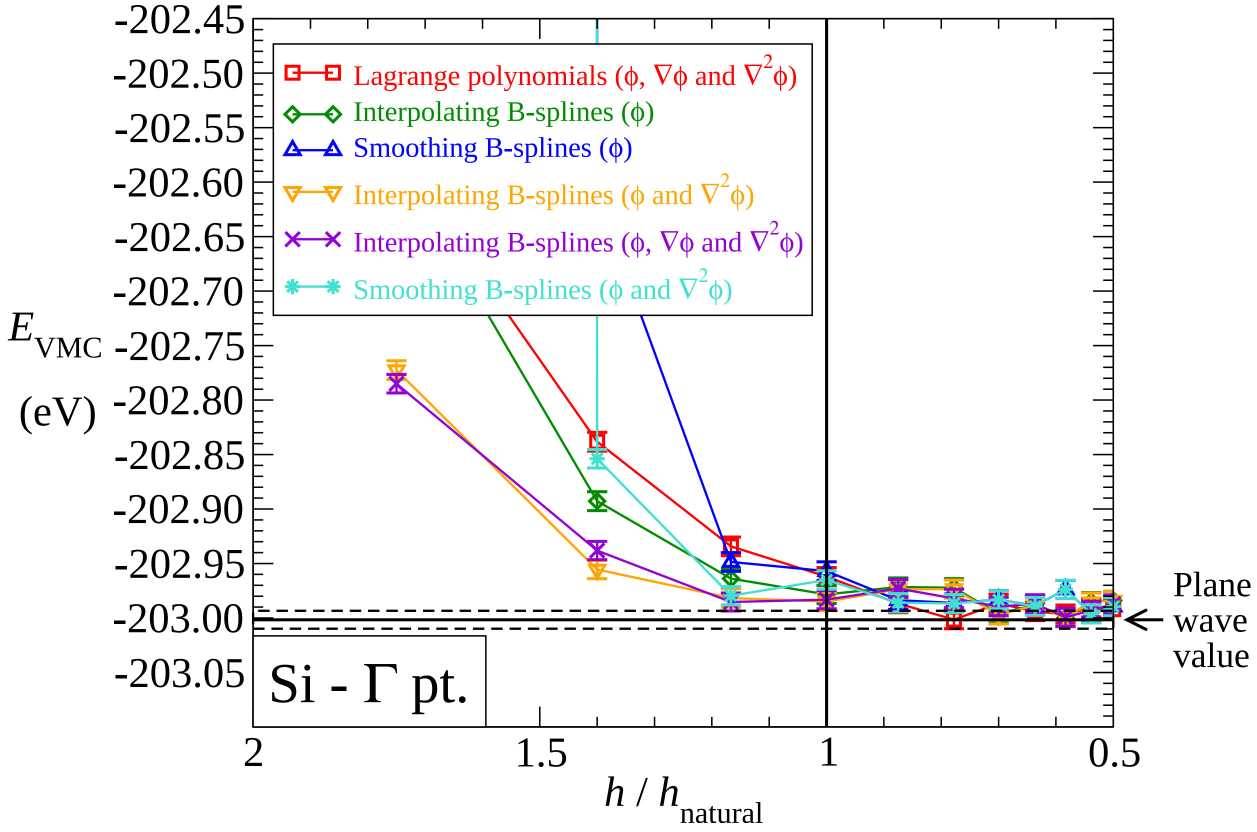


Figure II B 1: Convergence of planewave and approximation-method VMC energies in two-atom diamond Si at the Γ point with grid spacing (given as a ratio to natural grid spacing, defined in Equation 6 of the text). All methods show comparable convergence to the planewave value by natural grid spacing ($h/h_{\mathrm{natural}} = 1$).

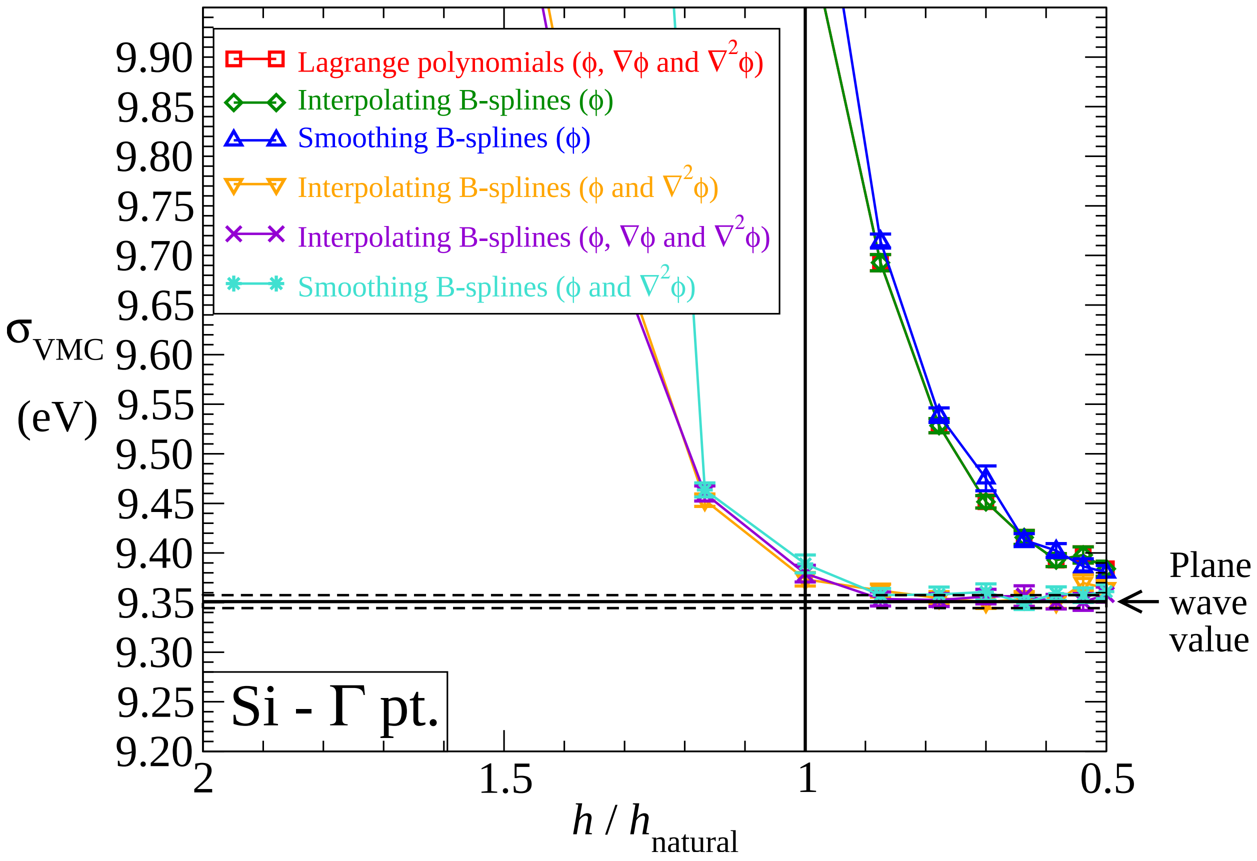


Figure II B 2: Convergence of planewave and approximation-method root-mean-square fluctuation in VMC energy of two-atom diamond Si at the Γ point with grid spacing (given as a ratio to natural grid spacing, defined in Equation 6 of the text). B-spline methods including direct approximation of the orbital Laplacian (those with $\nabla^2\phi$) show convergence to the planewave value at slightly finer than natural grid spacing. However, methods using derivatives of the approximation to calculate orbital Laplacian (those with $\phi$ alone) converge to the planewave value at much finer than natural grid spacing, requiring nearly twice as many grid points per direction. Lagrange polynomials, despite making a direct interpolation of the Laplacian, follow the trend of the B-splines without separate approximation for the Laplacian.

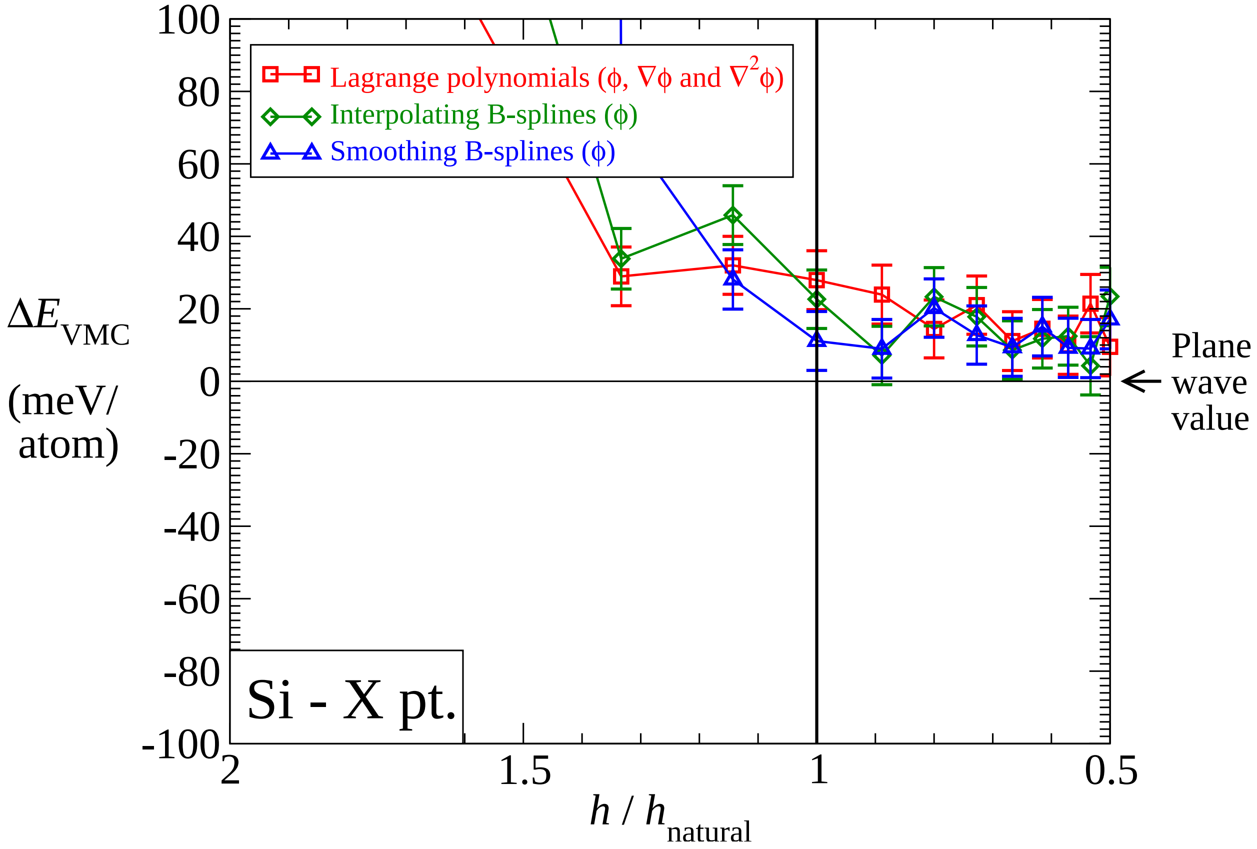


Figure II B 3: Convergence of the difference of approximation-method from planewave VMC energies in two-atom diamond Si at the X point with grid spacing (given as a ratio to natural grid spacing, defined in Equation 6 of the text). All methods show comparable convergence to the planewave value by natural grid spacing ($h/h_{\mathrm{natural}} = 1$) as they do at $\Gamma$ (see II B 1).

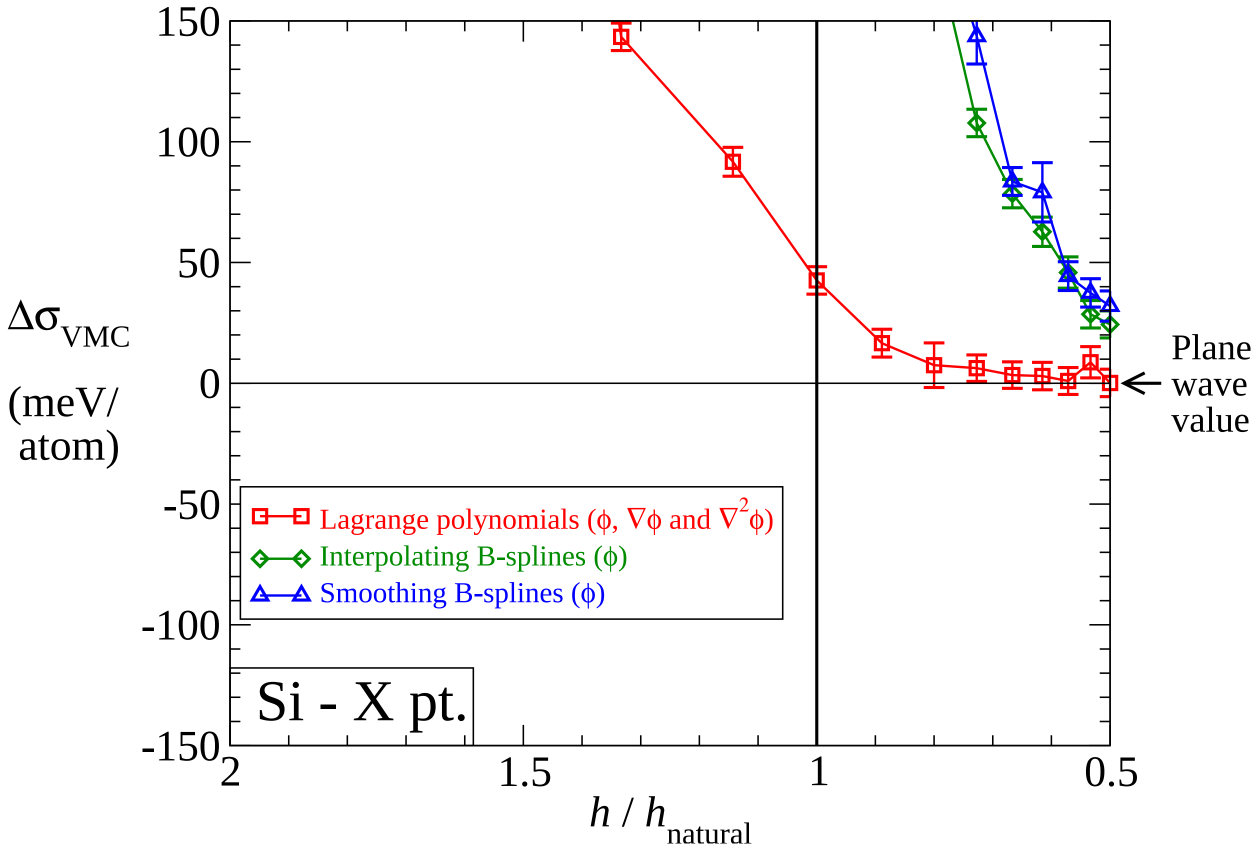


Figure II B 4: Convergence of the difference of approximation-method from planewave root-mean-square fluctuation in VMC energy of two-atom diamond Si at the X point with grid spacing (given as a ratio to natural grid spacing, defined in Equation 6 of the text). Unlike at Γ (see II B 1), Lagrange polynomials are nearly converged to the planewave value of RMS fluctuation at $h_{\text{natural}}$.

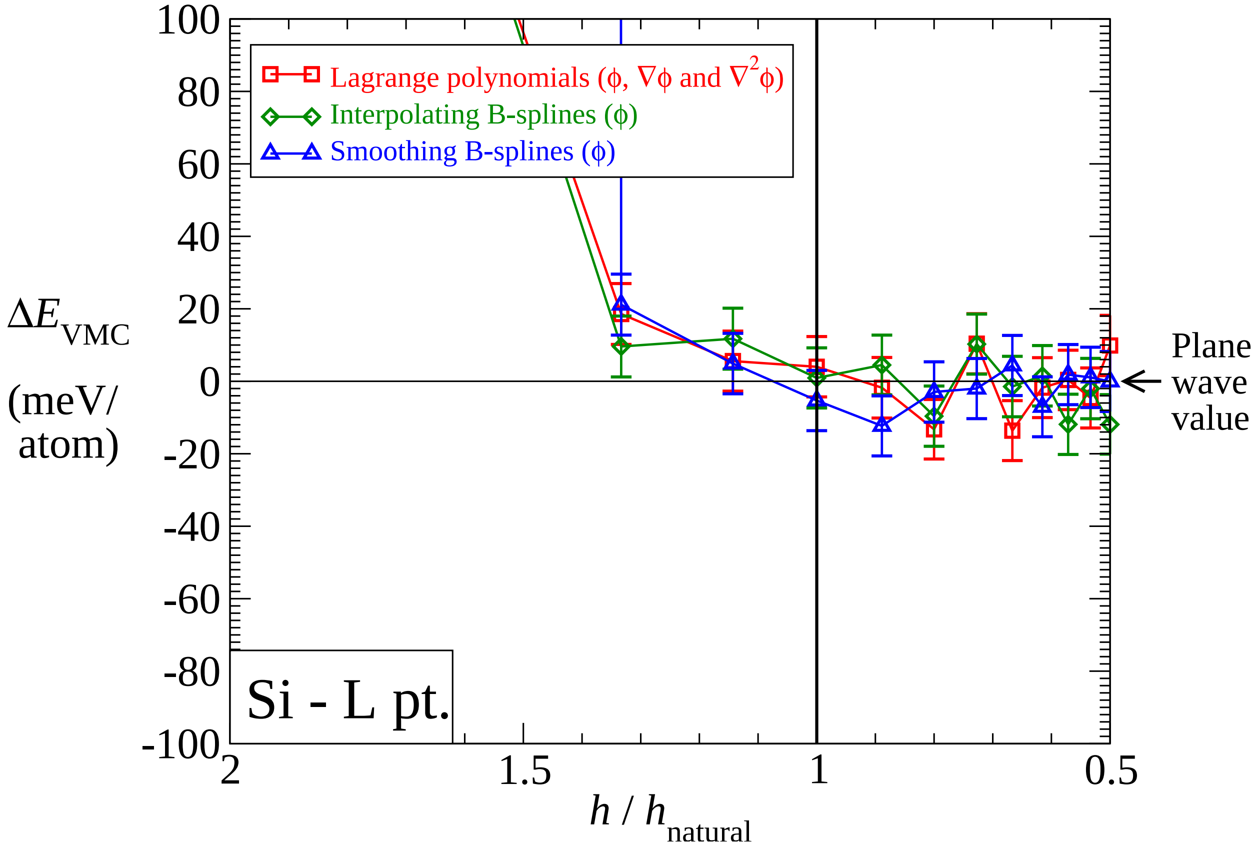


Figure II B 5: Convergence of the difference of approximation-method from planewave VMC energies in two-atom diamond Si at the L point with grid spacing (given as a ratio to natural grid spacing, defined in Equation 6 of the text). All methods show comparable convergence to the planewave value by natural grid spacing ($h/h_{\text{natural}} = 1$) as they do at $\Gamma$ (see II B 1).

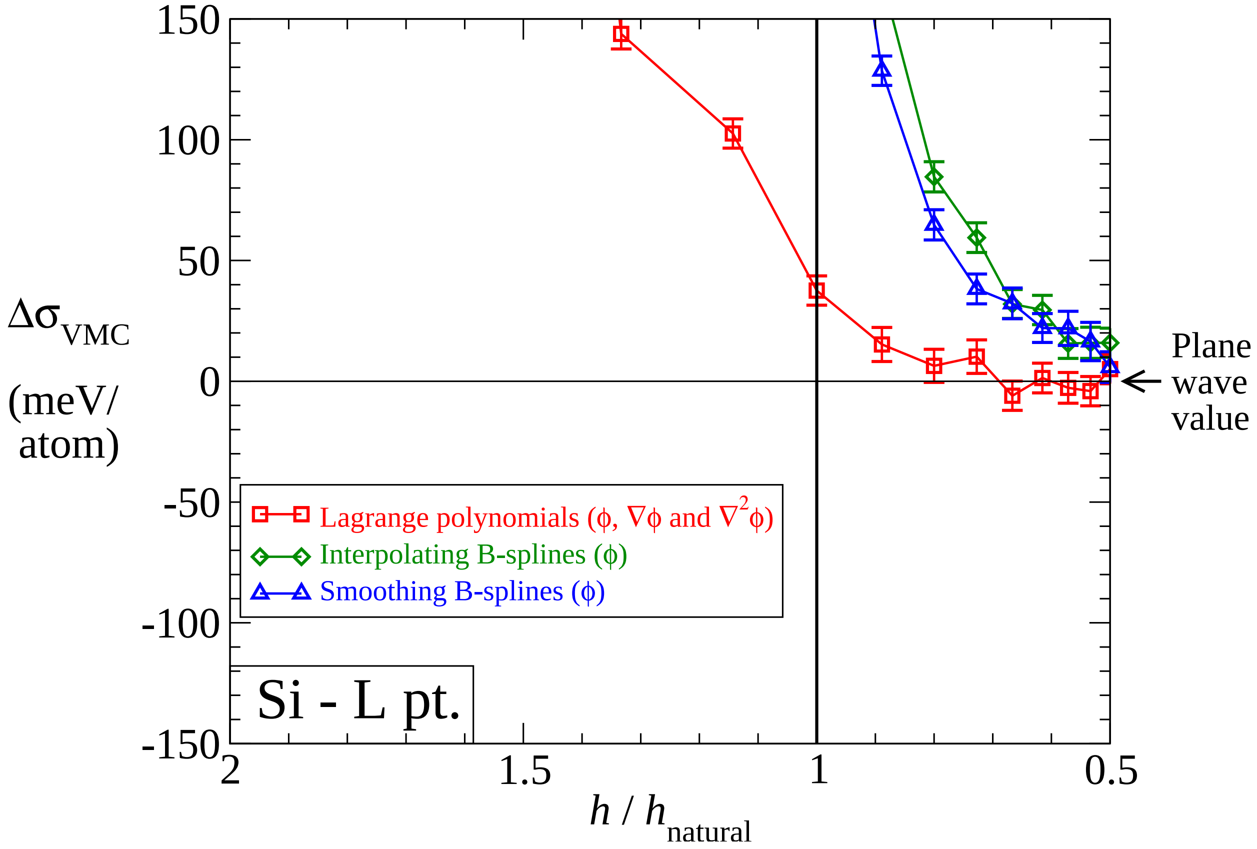


Figure II B 6: Convergence of the difference of approximation-method from planewave root-mean-square fluctuation in VMC energy of two-atom diamond Si at the L point with grid spacing (given as a ratio to natural grid spacing, defined in Equation 6 of the text). Unlike at Γ (see II B 1) but similar to X (see II B 3), Lagrange polynomials are nearly converged to the planewave value of RMS fluctuation at $h_{\mathrm{natural}}$.

## III. MAGNESIUM OXIDE

### A. Varying grid spacing

#### 1. VMC energy

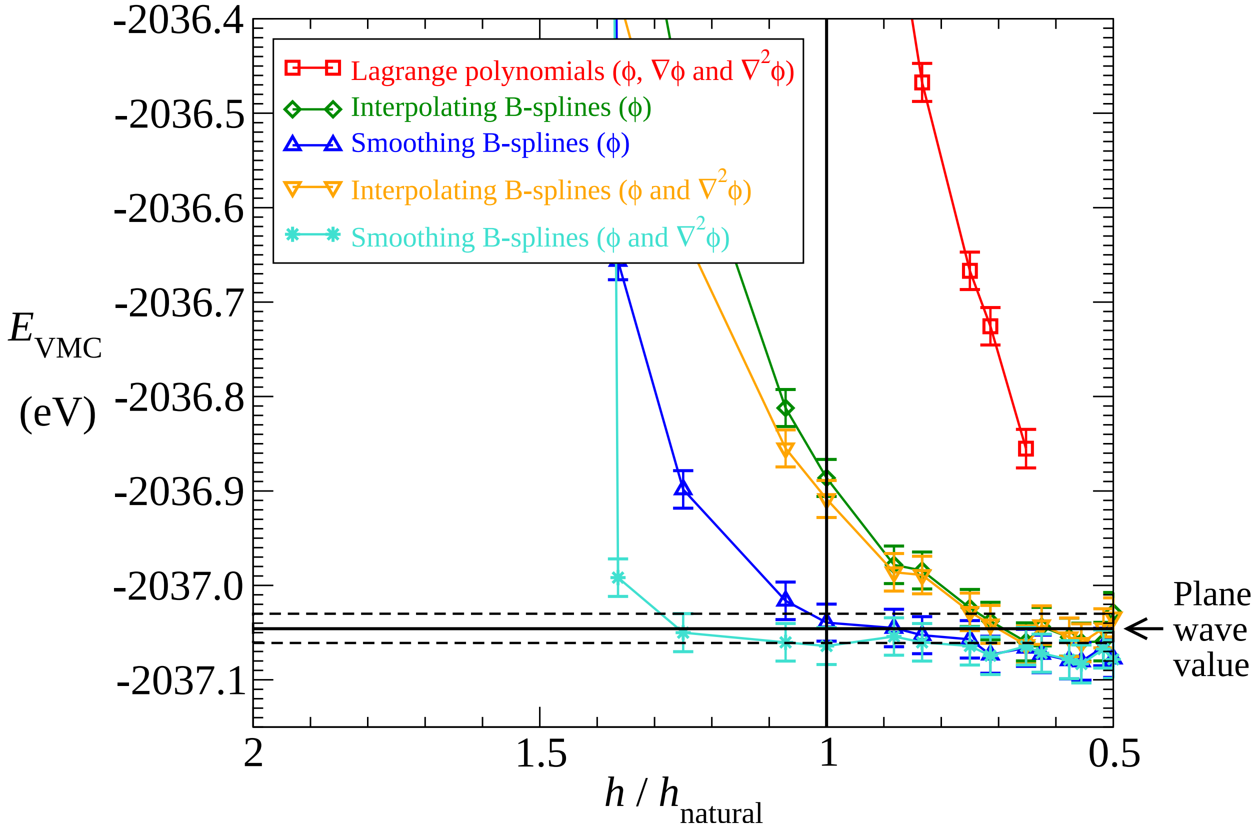


Figure III A 1: Convergence of planewave and approximation-method VMC energies in two-atom rock-salt MgO at the Γ point with grid spacing (given as a ratio to natural grid spacing, defined in Equation 6 of the text). Smoothing B-splines converge to the planewave value by $h_{\text{natural}}$ while interpolating B-splines do not converge until $\sim 3/4 h_{\text{natural}}$.

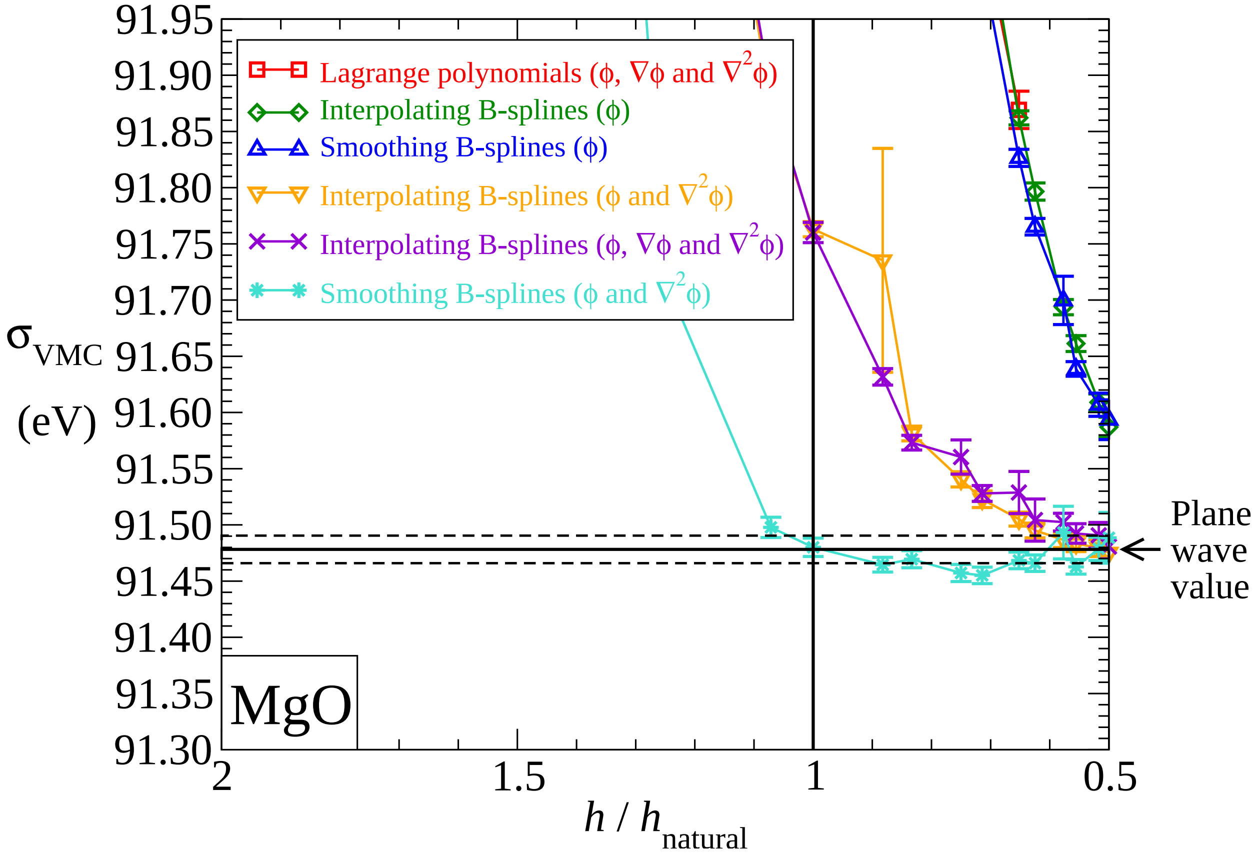


Figure III A 2: Convergence of planewave and approximation-method root-mean-square fluctuation in VMC energy of two-atom rock-salt MgO at the $\Gamma$ point with grid spacing (given as a ratio to natural grid spacing, defined in Equation 6 of the text). Only smoothing B-splines with a separate approximation for the Laplacian (those with $\nabla^2\phi$) converge to the planewave value for RMS fluctuation by $h_{\mathrm{natural}}$.
